# Supplementary material for: Panoptic-CUDAL: Rural Australia Point Cloud Dataset in Rainy Conditions
Source: arXiv:2503.16378 source file (2025-10-23)
Supplement: Supplementary file 1 [file 6_appendix.tex]

\section{Rain in datasets}

Rain poses significant challenges to LiDAR data collection, as it can substantially affect laser returns from wet surfaces.
Water on surfaces may cause laser beams to scatter or refract, altering return patterns and potentially impacting the accuracy and reliability of the point cloud.
For instance, puddles beneath objects may reflect the LiDAR’s laser, creating a shadow effect that can give the appearance of false objects below the ground surface.

Furthermore, the angle of incidence—the angle at which the laser beam hits a surface—can influence the reflectance and refraction of the laser, leading to variations in the point cloud.
High reflectance can cause the laser to scatter more, while low reflectance may result in weaker returns.
Both scenarios can introduce errors and distortions in the data.
Figure \ref{fig:lidar_outliers} illustrates these phenomena: on the left, a highly reflective object generates outlier points, while on the right, objects appear underground due to the reflection of the laser beams.

\begin{figure}[h!]
\centering
\includegraphics[width=0.99\columnwidth]{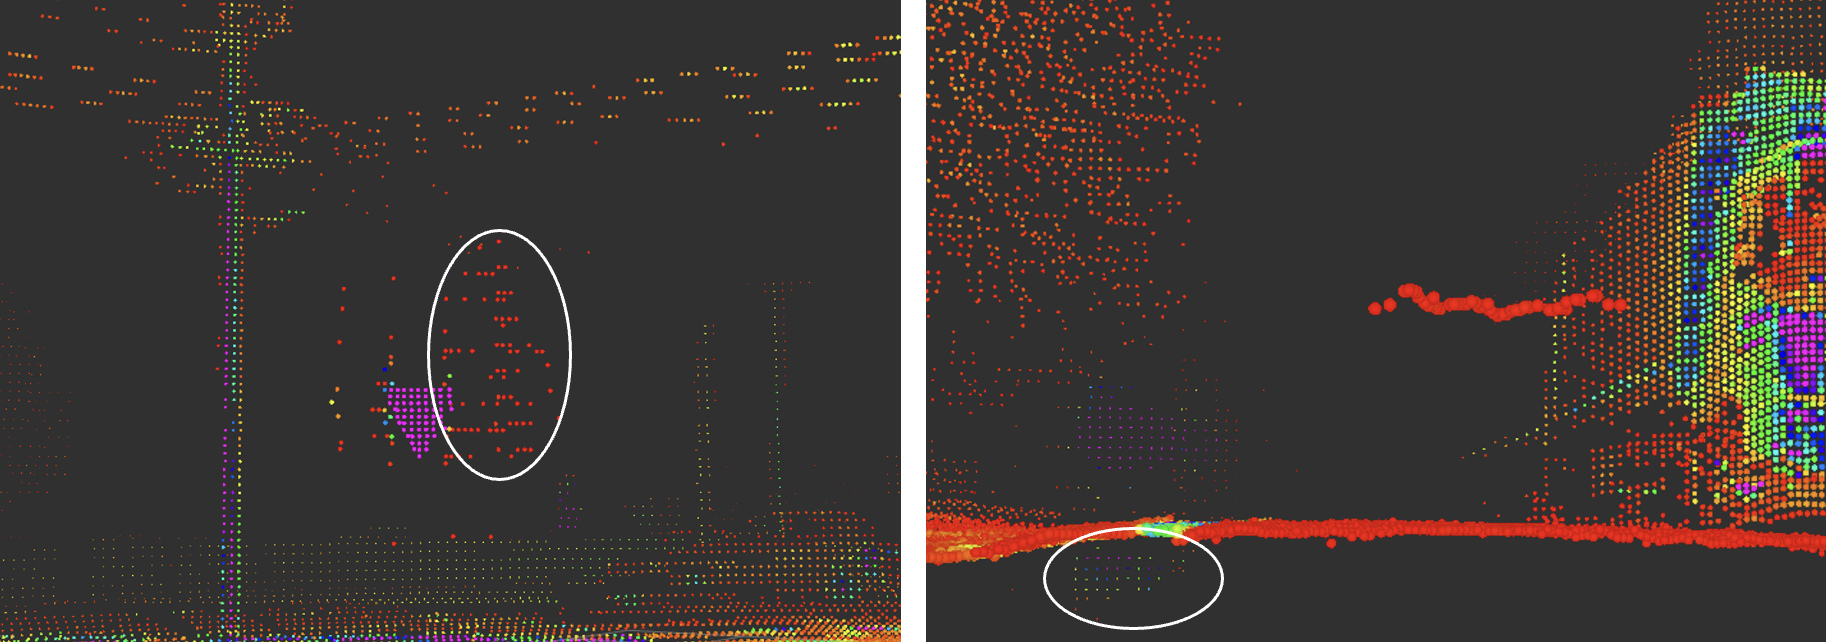}
\caption{\small Artifacts generated by the LiDAR due to its inherent operation are enclosed within the white ellipse.}
\label{fig:lidar_outliers}
\end{figure}

Moreover, water droplets and splashes can cause laser beams to scatter and refract unpredictably.
This scattering can lead to multiple reflections and diffuse returns, generating points that do not accurately represent the physical environment.
This effect increases the overall noise and can obscure or distort nearby objects.
For example, when a car passes by and splashes water from its tires, the splashed water creates numerous small droplets in the air, which reflect the LiDAR laser beams and are captured as points in the point cloud, introducing spurious points that do not correspond to any solid objects.
The dynamic nature of splashes introduces fast-changing noise patterns, making it difficult to filter and denoise. 

\begin{figure}[h!]
\centering
\includegraphics[width=0.98\columnwidth]{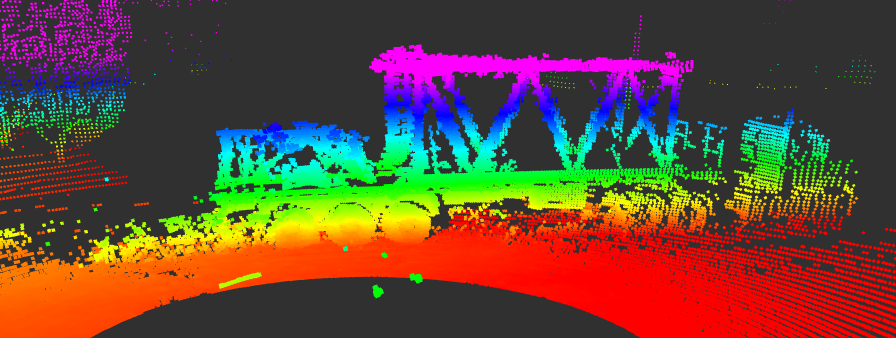}
\caption{\small A heavy truck splashing water from its rear end and the resulting point cloud generated by the LiDAR returns.}k\label{fig:splash}
\end{figure}

Understanding the influence of environmental factors is vital for accurately analyzing LiDAR data collected under varying weather conditions and in rural areas.
As observed, environmental variables can significantly impact point cloud data, underscoring the importance of data collection and annotation that incorporate these variations for effective point cloud analysis.

 Consequently, the annotations derived from this data offer invaluable insights to the research community, informing the development of more adaptable and robust autonomous driving technologies capable of navigating less structured settings.
